# Supplementary material for: Tiramisu: A Polyhedral Compiler for Expressing Fast and Portable Code
Source: arXiv:1804.10694 source file (2018-12-20)
Supplement: Supplementary file 1 [file appendix.tex]

\section{Notation and Definitions}

\subsection{Presburger formula\label{presburger}}

We use an EBNF (Extended Backus-Naur Form) grammar to define Presburger formulas.
\[
\begin{array}{lcl}
\pgrammar{formula} & \gets &  \pgrammar{formula} \wedge \pgrammar{formula} \\ 
        & & ~|~ \pgrammar{formula} \vee   \pgrammar{formula} \\
        & & ~|~ \neg \pgrammar{formula} 
        ~|~ \exists \pgrammar{var}. \pgrammar{formula} \\
        & & ~|~ \forall \pgrammar{var}. \pgrammar{formula}
        ~|~ \pgrammar{atom} \\
                            
\pgrammar{atom} & \gets &  \pgrammar{term} \pgrammar{relop} \pgrammar{term}
                            \\
\pgrammar{term} & \gets &     \pgrammar{numeral}
        ~|~ \pgrammar{term} + \pgrammar{term} \\
        & & ~|~ -\pgrammar{term} \\
        & & ~|~ \pgrammar{numeral} * \pgrammar{term}
        ~|~ \pgrammar{var}
                            \\
\pgrammar{relop} & \gets &    <
        ~|~ \leq
                            ~|~ =
                            ~|~ >
                            ~|~ \geq
                            \\
\pgrammar{var} & \gets &      x
                            ~|~ y
                            ~|~ z
                            ~|~ \dots
                            \\
\pgrammar{numeral} & \gets &  0
                            ~|~ 1
                            ~|~ 2
                            ~|~ \dots
                            \\
\end{array}
\]

Note that $\pgrammar{numeral} * \pgrammar{term}$ is not a general multiplication operator;
it is a shortcut for $\pgrammar{term}+\dots+\pgrammar{term}$.

Presburger arithmetic is used mainly because it is a decidable arithmetic.
That is, there exists an algorithm which decides whether an arbitrary Presburger formula is true (valid) or not, which is important for many polyhedral operations.

\subsection{Quasi-Affine Constraints}
\label{qaffine}

A \emph{quasi-affine constraint} is a constraint over integer values and integer variables involving only the operators \lstinline{+}, \lstinline{-}, $\times$, \lstinline{/}, \lstinline{mod}, \lstinline{&&}, \lstinline{||}, \lstinline{<}, \lstinline{<=}, \lstinline{>}, \lstinline{>=}, \lstinline{==}, \lstinline{!=}, and the ternary \lstinline{?:} operator, where the second argument of \lstinline{/} and \lstinline{mod} must be a (positive) integer literal, and where at
least one of the arguments of $\times$
must be a constant expression.
An example of a quasi-affine constraint for a statement in a loop nest is $10\times i+j+n>0$, where $i$ and $j$ are loop iterators and $n$ is a
\emph{symbolic constant} (i.e., a variable that has an unknown but fixed value for the duration of
an execution).  An example of a non-quasi-affine constraint is $i \times i>0$, because we require one of the arguments be a constant.

\section{Integer Sets}

An \emph{integer set} is a set of integer tuples from $\mathbb{Z}^d$ that can be specified using  affine constraints. $d$ is the dimensionality of the set (the number of integers in each tuple) and a d-tuple is represented as $(a_1, a_2, \dots, a_d)$.  An example of a set of integer tuples is:
$$\{(1,1); (2,1); (3,1); (1,2); (2,2); (3,2)\}$$

Instead of listing all the integer tuples of the set, we describe the set using affine constraints:
$$\{S(i,j): 1 \leq i \leq 3 \wedge 1 \leq j \leq 2\}$$

\noindent where $i$ and $j$ are the dimensions of the set.
The tuples of a set can optionally have a common name, such as
$S$ in this example.
Figure~\ref{fig:set} shows a graphical representation of the map $S$.

\begin{figure}[th]
  \begin{minipage}{.22\textwidth}
    \centering
    \includegraphics[scale=0.6]{figures/set.pdf}
    \captionof{figure}{Graphical representation of a set}
    \label{fig:set}
  \end{minipage}
  \begin{minipage}{.22\textwidth}
    \centering
    \includegraphics[scale=0.6]{figures/map.pdf}
    \captionof{figure}{Graphical representation of a map}
    \label{fig:map}
  \end{minipage}
\end{figure}

In general, an integer set has the form
$$S = \{N(\vec{s}) | f(\vec{s}, \vec{p})\}$$

\noindent with $\vec{s}$ representing the integer tuples of
the integer set ($\vec{s} \in \mathbb{Z}^d$), $N$, a common name
for all the tuples $\vec{s}$ usually used as the name of computations, $d$ the dimensionality of the set, $\vec{p} \in \mathbb{Z}^e$ a vector of $e$ parameters and $f(\vec{s}, \vec{p})$ a Presburger formula that evaluates to true, if and only if $\vec{s}$ is an element of $S$ for the given parameters $\vec{p}$.

\subsection{Relations (maps)}
A map is a relation between two integer sets.  For example
$$M = \{S1(i,j) \rightarrow S1(i+2,j+2) : 1 \leq i \leq 3 \wedge 1 \leq j \leq 2\}$$

\noindent represents a relation between two sets. The first set
is called the \emph{domain} or the \emph{source}
and the second is called the \emph{range} or the
\emph{sink}.
Figure~\ref{fig:map} shows a graphical representation of
the map $M$.

In general, a map has the form
$$M = \{A(\vec{s}) \rightarrow B(\vec{o}), (\vec{s}, \vec{o}) \in \mathbb{Z}^{d_1}\times\mathbb{Z}^{d_2} | f(\vec{s}, \vec{o}, \vec{p})\}$$

\noindent where $A(\vec{s})$ represents the domain or the
source and $B(\vec{o})$ represents the range or the sink.
$d_1$ and $d_2$ are the dimensionalities of $\vec{s}$
and $\vec{o}$, $\vec{p} \in \mathbb{Z}^e$ is a vector of $e$ parameters and $f(\vec{s}, \vec{o}, \vec{p})$ is a Presburger formula that evaluates to true if and only if there is a relation from $\vec{s}$ to $\vec{o}$ in $M$ for the given parameters
$\vec{p}$.

%\section{Three-Layer IR}
%\label{appendixlayers}
%\subsection{Layer I: \Layerone}

%The first layer is a union of \emph{computation sets} such that each computation set describes one statement in the program. Each computation set is defined as follows:
%$$\{N1(\vec{s}) | f(\vec{s}, \vec{p})\} : g(N2(\vec{s}), N3(\vec{s}), ..., N4(\vec{s}))$$

%\noindent where $N1(\vec{s})$ is a computation that has the name $N1$, and where $g(N2(\vec{s}), N3(\vec{s}), ..., N4(\vec{s}))$ is the expression that the computation computes and $f(\vec{s}, \vec{p})$ is a Presburger formula that evaluates to true, if and only if $\vec{s}$ is an element of $S$ for the given parameters $\vec{p}$.

%\subsection{Layer II: \Layertwo}

%The second layer is identical to the first layer except that computations in this layer are ordered based on their lexicographical order.

%\subsection{Layer III: \Layerthree}
%\label{layer3}

%The third layer is a union of computation sets and a set of access relations.  The computation sets are identical to the Layer II computation sets except that new allocation/deallocation statements are added.  The set of access relations is described as follows:
%$$\{N1(\vec{s}) \rightarrow B(\vec{o}), (\vec{s}, \vec{o}) \in \mathbb{Z}^{d_1}\times\mathbb{Z}^{d_2} | f(\vec{s}, \vec{o}, \vec{p})\}$$

%\noindent where $N1(\vec{s})$ is a computation mapped to the buffer element $B[\vec{o}]$ and $f(\vec{s}, \vec{o}, \vec{p})$ is a Presburger formula that evaluates to true if and only if there is a relation from $\vec{s}$ to $\vec{o}$ for the given parameters $\vec{p}$.

\section{Example}

Figure~\ref{fig:time-processor-vector} provides examples of different optimizations expressed in Layer II.

\begin{figure}
\small

\centering\begin{lstlisting}[language=C,escapechar=@,basicstyle=\linespread{0.9}\small\ttfamily]
for (i in 0..N)
  for (j in 0..M)
    S1
    S2
\end{lstlisting}
(a) Original computation expressed as an imperative program

\begin{tabular}{c|c}
\\\hline
   \begin{tabular}{l@{\hspace{4pt}}r@{\hspace{2pt}}c@{\hspace{2pt}}c@{\hspace{2pt}}c@{\hspace{0pt}}l}
    S1: & ( & $i,$ & $j$, & $0$ & ) \\
    S2: & ( & $i$, & $j$, & 1 & ) \\
    \multicolumn{6}{c}{ (b) Sequential}
   \end{tabular}
     &  
   \begin{tabular}{l@{\hspace{4pt}}r@{\hspace{2pt}}c@{\hspace{2pt}}c@{\hspace{2pt}}c@{\hspace{0pt}}l}
    S1: & ( & $j$, & $i$, & 0 & ) \\
    S2: & ( & $j$, & $i$, & 1 & ) \\
    \multicolumn{6}{c}{ (c) Transposed}
   \end{tabular} \\\hline

    \begin{tabular}{l@{\hspace{4pt}}r@{\hspace{2pt}}c@{\hspace{2pt}}c@{\hspace{2pt}}c@{\hspace{0pt}}l}
    S1: & ( & $i$, & 0, & $j$ & ) \\
    S2: & ( & $i$, & 1, & $j$ & ) \\
    \multicolumn{6}{c}{ (d) Inner loop fission}
   \end{tabular} 
   & 
    \begin{tabular}{l@{\hspace{4pt}}r@{\hspace{2pt}}c@{\hspace{2pt}}c@{\hspace{2pt}}c@{\hspace{0pt}}l}
    S1: & ( & 0, & $i$, & $j$ & ) \\
    S2: & ( & 1, & $i$, & $j$ & ) \\
    \multicolumn{6}{c}{ (e) Outer loop fission}
   \end{tabular} \\\hline
   
    \begin{tabular}{l@{\hspace{4pt}}r@{\hspace{2pt}}c@{\hspace{2pt}}c@{\hspace{2pt}}c@{\hspace{2pt}}c@{\hspace{0pt}}l}
    S1: & (  & $i/N$, & $i\%N$, & $j$, & 0 & ) \\
    S2: & (  & $i/N$, & $i\%N$, & $j$, & 1 & ) \\
    \multicolumn{6}{c}{ (f) Loop split}
   \end{tabular} 
   &
    \begin{tabular}{l@{\hspace{4pt}}r@{\hspace{2pt}}c@{\hspace{2pt}}c@{\hspace{2pt}}c@{\hspace{2pt}}c@{\hspace{0pt}}l}
    S1: & ( & $i/N$, & $j$, & $i\%N$, & 0 & ) \\
    S2: & ( & $i/N$, & $j$, & $i\%N$, & 1 & ) \\
    \multicolumn{6}{c}{ (g) ... \& permuted}
    \end{tabular}  \\\hline
    
    \begin{tabular}{l@{\hspace{4pt}}r@{\hspace{2pt}}c@{\hspace{2pt}}c@{\hspace{2pt}}c@{\hspace{2pt}}c@{\hspace{0pt}}l}
    S1: & ( & $i\%P$ {\it (cpu)}, & $j$, & $i/P$, & 0 & ) \\
    S2: & ( & $i\%P$ {\it (cpu)}, & $j$, & $i/P$, & 1 & ) \\
    \multicolumn{6}{c}{ (h) Outer parallel }
   \end{tabular} 
   &
    \begin{tabular}{l@{\hspace{4pt}}r@{\hspace{2pt}}c@{\hspace{2pt}}c@{\hspace{2pt}}c@{\hspace{2pt}}c@{\hspace{0pt}}l}
    S1: & ( & $i$, & $j/4$, & 0, & $j\%4$ {\it (vec)} & ) \\
    S2: & ( & $i$, & $j/4$, & 1, & $j\%4$ {\it (vec)} & ) \\
    \multicolumn{6}{c}{ (i) Inner vectorized }
   \end{tabular} \\ 

\end{tabular}
 \caption{For a simple loop next with two statements, examples of different time-processor vectors leading to many possible execution arrangements. }
\label{fig:time-processor-vector}
\end{figure}

\section{Julia to \framework{}}

\subsection{Transforming Julia to \framework{}}

Julia is a high-level dynamically-typed programming language designed for numerical computing.  
However, in contrast to Halide, Julia is more general: it supports while loops and recurrent computations and is memory-based (i.e., it uses variables unlike Halide which defines pure functions mostly).
We extend Julia with a set of scheduling directives and function annotations.  Functions annotated with the \lstinline{@acc} macro are optimized with \framework{}.

\framework{} is designed mainly for optimizing sequences of loop nests and statements manipulating arrays.  The user annotates which julia function should be translated; this function can only contain foor loops and statements manipulating arrays.
We generate \framework{} from the low-level Julia IR (which is in SSA form) by translating each statement in the Julia IR into a computation in \framework{}.  This Julia low-level IR does not have high level control flow (it only has \lstinline{gotos}); thus we change the compilation flow of Julia to annotate the low-level IR with information about the original control flow of the program.  We use the annotations to recover the control flow and generate the iteration domain of each computation.  Although Julia has another high level IR that has control flow information, we cannot use that IR because it lacks the necessary data type annotations.

We transform the memory-based Julia IR into the producer-consumer \framework{} IR using classical array expansion techniques~\cite{feautrier_array_1988,midkiff_automatic_2012,maydan_array-data_1993}.  The goal here is to extract the data-flow representation of the code.  The user is then free to change the data layout of computations using high level data-layout directives. % The problem of array expansion 

\subsection{Evaluating Julia to \framework}

\begin{figure}
\centering
 \includegraphics[width=0.8\columnwidth]{./figures/tiramisu_vs_julia}
 \caption{Execution Time for \framework and Julia (s)}
 \label{fig:speedup_julia}
 \vspace{-0.5cm}
\end{figure}

We used the following benchmarks to evaluate the integration of \framework within Julia: \texttt{bicg}, a biconjugate gradient method;  \texttt{doitgen}, a multiresolution analysis kernel;  \texttt{mttkrp}, the matricized tensor times Khatri-Rao product; \texttt{covariance}, which performs a covariance computation; and \texttt{gesummv}, which is summed matrix-vector multiplications.
For a fair comparison, the Julia code was tagged with the \texttt{inbounds} macro to remove any boundary checks on buffer accesses. 

Figure~\ref{fig:speedup_julia} shows the execution time of code generated by Julia-\framework{} compared to Julia without \framework{}.  The speedups of Julia-\framework{} in \texttt{covariance}, \texttt{doitgen}, \texttt{mttkrp} and \texttt{bicg} are mainly due to the improved data locality obtained after tiling using \framework{}, which is not possible in Julia.
